# Supplementary material for: Adv3D: Generating 3D Adversarial Examples for 3D Object Detection in Driving Scenarios with NeRF
Source: arXiv:2309.01351 source file (2024-08-06)
Supplement: Supplementary file 1 [file 08_supp.tex]

\appendix
% \section*{\centering Supplementary Material for\\ Adv3D: Generating 3D Adversarial Examples for 3D Object Detection in Driving Scenarios with NeRF}
% \vspace{4mm}

\section{Overview}\label{overview}

This supplementary material is organized as follows:

\begin{itemize}
    \item We first provide training details of our adversarial examples in Sec.~\ref{training_detail}. We then detail the sampling pose distribution $\mathcal{B}$ in Sec.~\ref{sample_pose_para}.
    \item In Sec.~\ref{supp_real_exp}, we demonstrate the attack effectiveness of reproducing the adversarial texture in our real world. 
    \item We provide analysis and ablation studies on the number of adversarial examples in Sec.~\ref{num_adv}, and evaluate the transferability of adversarial texture to the unseen vehicle in Sec.~\ref{trans_unseen}. 
    \item Finally, we provide repeatability tests in Sec.~\ref{repe_test}, investigate the influence of perceptibility of the attack in Sec.~\ref{perceptibility}, and present additional qualitative results in Sec.~\ref{qua_result}. We discuss limitations and future work in Sec.~\ref{sec:limit}.
    
    % In our experiments in the supplementary material, we use BEVDet~\cite{huang2021bevdet} as the attacked 3D detector.
\end{itemize}

\section{Training Details}\label{training_detail}
We implement our methods using PyTorch~\cite{paszke2019pytorch} and MMDetection3D~\cite{mmdet3d2020}. All detectors are resumed from checkpoints available on their open-source repositories to match the original performance exactly. We only select one instance from Lift3D~\cite{lift3D2023CVPR} as the initialization of examples. We conduct our experiments using 8 NVIDIA A100 80G GPUs. We use the Adam optimizer~\cite{kingma2014adam} with a learning rate of 1e-3 for texture latents. In practice, we optimize texture latents on the training set for five epochs with the same batch size as used during training detectors. We do not use any regularization except for semantic-guided regularization. In all experiments without specified, we render two adversarial examples per image.

\section{Sampling Pose Distribution}\label{sample_pose_para}
In this section, we introduce the distribution of pose $\mathcal{B}$ used during pose sampling. Specifically, we parameterize the pose $\mathcal{B}$ as 3D bounding boxes that are described by $(x,y,z,l,w,h,\theta)$, where $x, y, z$ is the position of the 3D bounding box's center, $l, w, h$ represent length, width, height of the box, $\theta$ is the rotation along $y$ axis. As shown in Tab.~\ref{tab:sam_param}, we model the components of $\mathcal{B}$ as independently sampled parameters. We mainly follow the parametrization in Lift3D~\cite{lift3D2023CVPR}.

To avoid inappropriate sampling in driving scenes (such as a car flying in the sky), we model our objects to roughly be placed on a ground plane in front of the camera. To approximate the ground plane, we set $(x,z)$ to be uniformly sampled from $[-5m, 5m]$ and $[10m, 15m]$. As for $y$, we first obtain camera height from the camera extrinsic, then we model $y$ as a Gaussian distribution that is centered at the camera height. Similarly, $l_{mean}$, $w_{mean}$, and $h_{mean}$ is the mean value of length, width, and height of the 3D box obtained from the statistic of datasets, where $l_{mean}=4.61m, w_{mean}=1.95m, h_{mean}=1.72m$. Then we model the size of 3D boxes as a Gaussian distribution that is centered at the mean value. The rotation of the object is considered as a bimodal distribution that is centered at forward facing($\pi / 2$) and backward facing($-\pi / 2$).

\begin{table}[h]
    \centering
    % \vspace{-1.0mm}
        % \resizebox{\textwidth}{!}{

    \begin{tabular}{lcccccc}
    \toprule
    \textbf{Pose} & \textbf{Distribution} &  \textbf{Parameters}   \\
    \midrule
    $x$ & Uniform  & $[-5m, 5m]$  \\
    $y$ & Gaussian  & $\mu = height, \sigma = 0.2$  \\
    $z$ & Uniform  & $[10m, 15m]$  \\
    $l$ & Gaussian  & $\mu = l_{mean}, \sigma = 0.5$  \\
    $w$ & Gaussian  & $\mu = w_{mean}, \sigma = 0.5$  \\
    $h$ & Gaussian  & $\mu = h_{mean}, \sigma = 0.5$  \\
    $\theta$ & Gaussian  & $\mu = \pm \pi / 2, \sigma = \pi / 2$  \\
    \bottomrule
    \end{tabular}
        % \vspace{-.7em}
        % }
    \caption{Detailed distribution of pose $\mathbf{b}$ in pose sampling.}
    % \vspace{-.1em}
    \label{tab:sam_param}
\end{table}

\begin{figure*}[h!]
    \centering
    \includegraphics[width = 1\textwidth, trim = 0 0 0 0, clip]{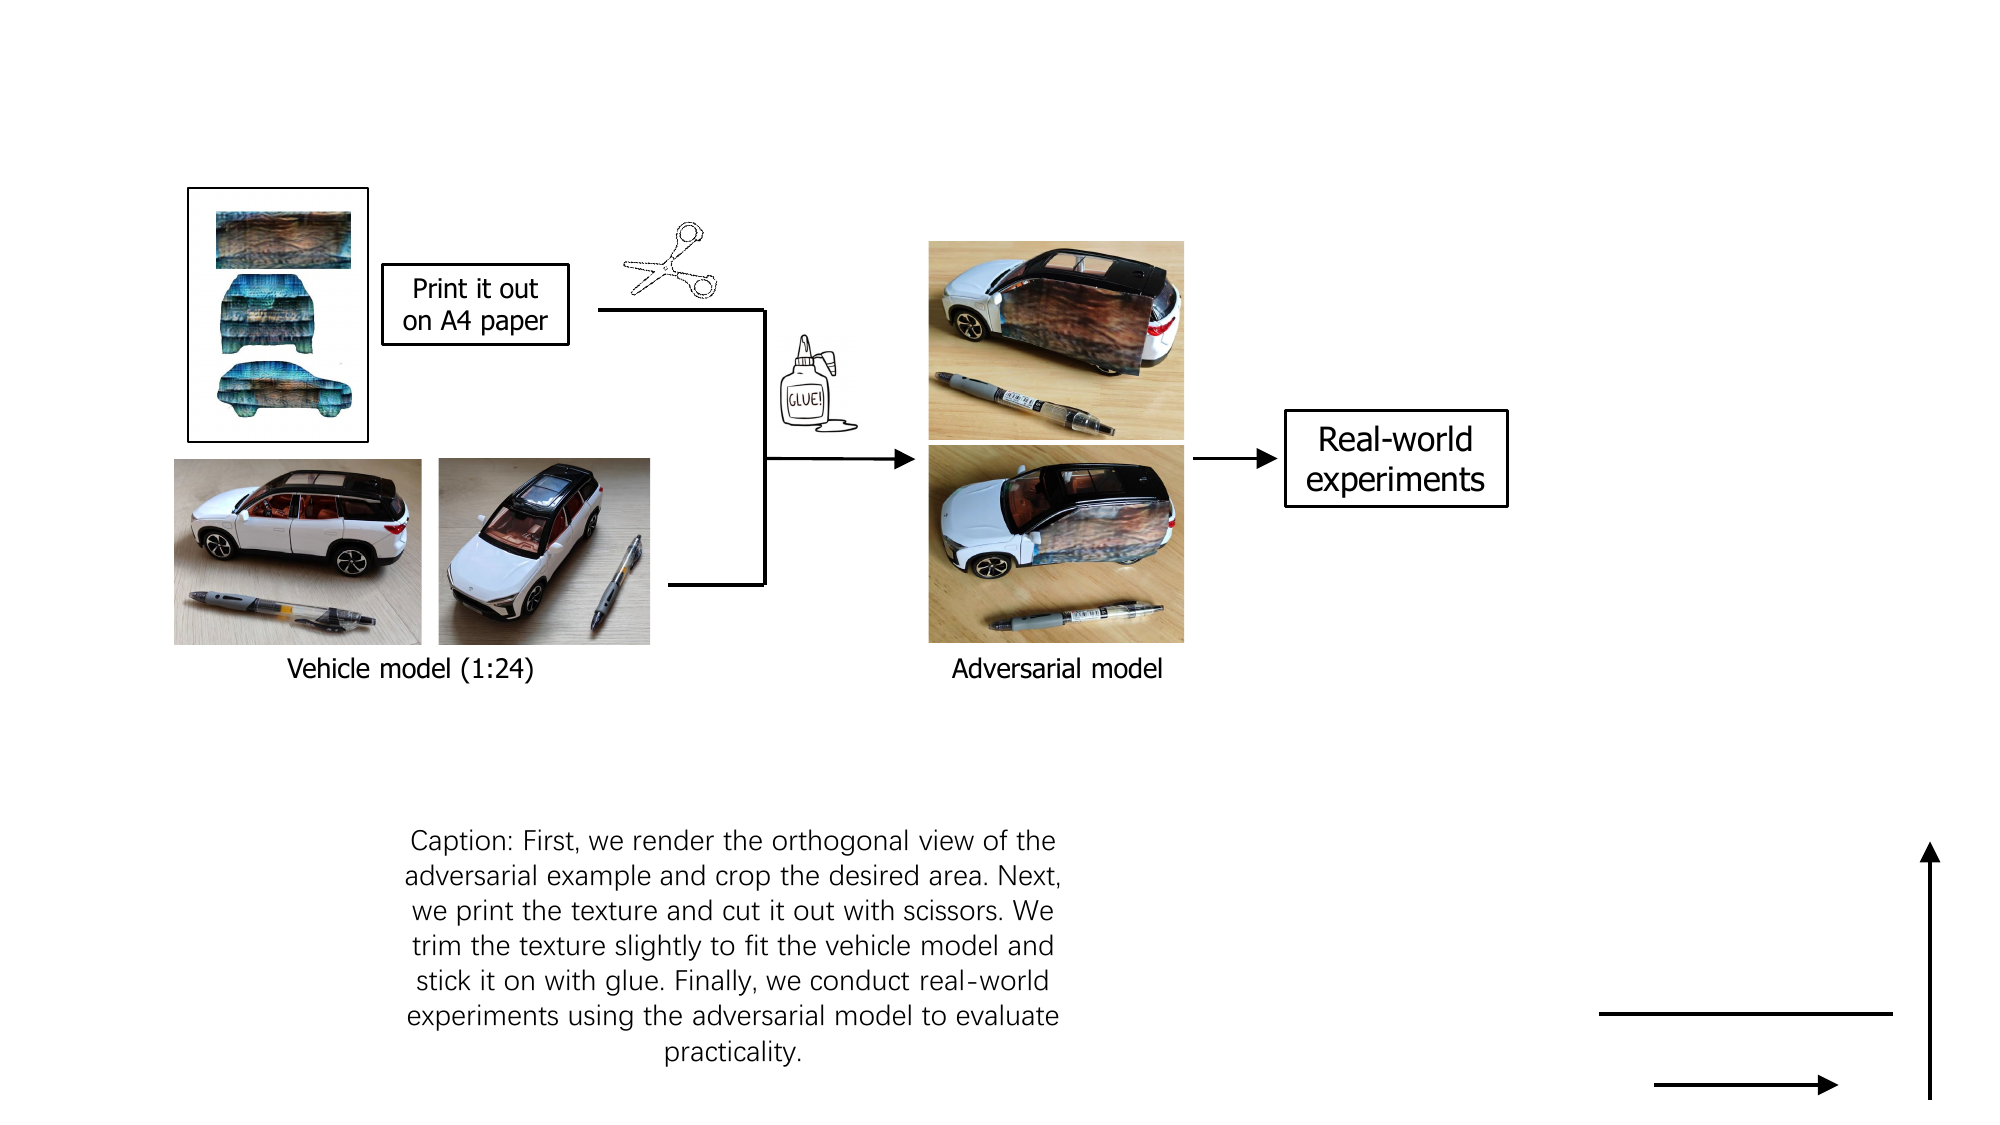}
   \caption{\textbf{Setup of real-world experiments.} 
    }
    \label{fig:real_exp_setup}
\end{figure*}

\begin{figure*}[h!]
    \centering
    \includegraphics[width = 1\textwidth, trim = 0 0 0 0, clip]{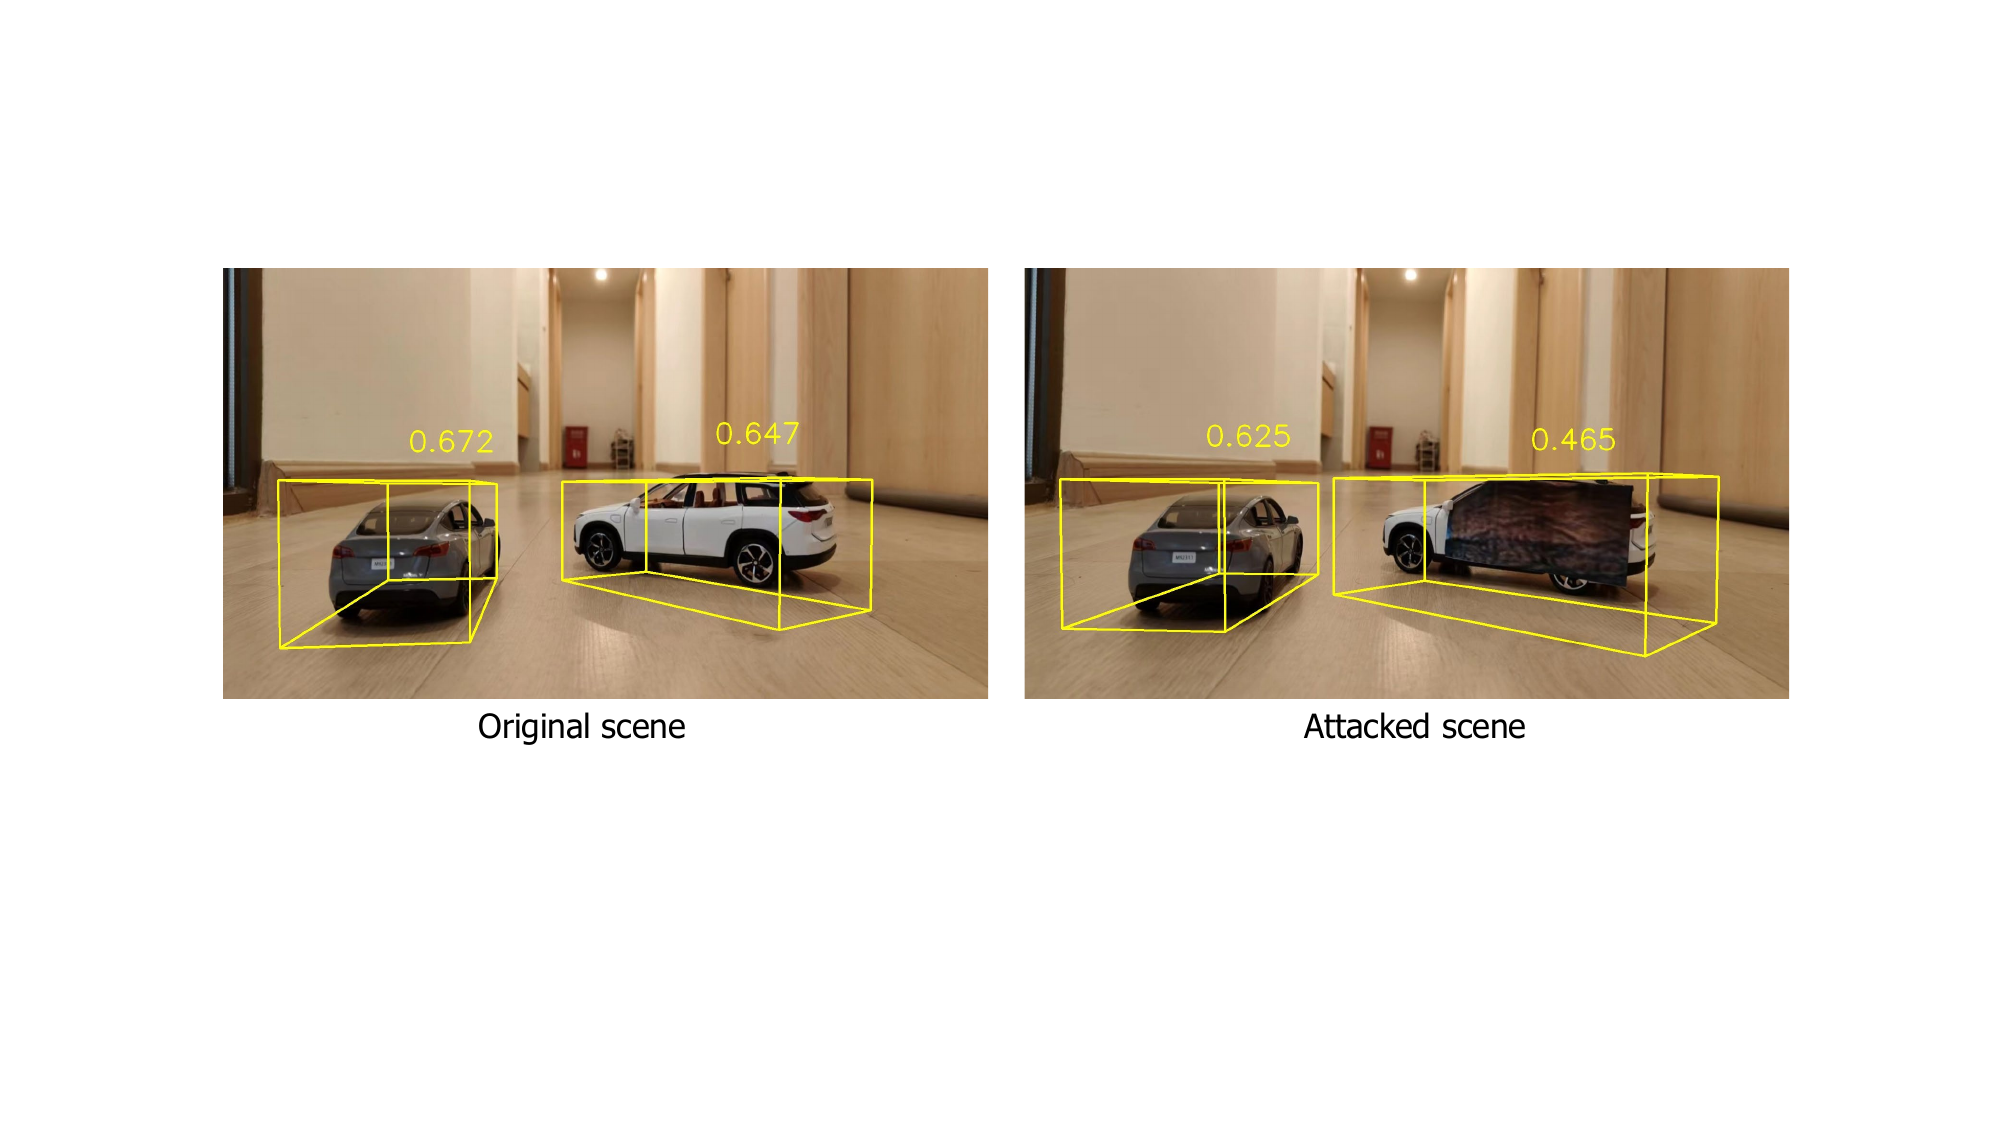}
   \caption{\textbf{Results of real-world experiments.} Note that the result is achieved without fine-tuning in the current scene.
    }
    \label{fig:real_exp_result}
\end{figure*}

\section{Reproduce 3D Adversarial Examples in Real-World}\label{supp_real_exp}

As depicted in Fig.~\ref{fig:real_exp_setup}, we reproduce our adversarial scene in the real world by creating a scaled driving scene using 1:24 vehicle models. We approximate the adversarial textures using the rendering of the orthogonal views of examples. We first crop the desired area from the orthogonal view of adversarial example. Next, we print the texture on A4 paper and cut out the desired shape using scissors. We then trim the texture slightly to fit the vehicle model and adhere to it using glue. 

% Afterward, we conduct real-world experiments using the adversarial model to evaluate its practicality.

After reproducing the adversarial example in our real world, we use it to attack BEVDet~\cite{huang2021bevdet} in our created scene, as shown in Fig.~\ref{fig:real_exp_result}. In our experiment, only the front view images are replaced with the attacked images, while the other five surround view images are sampled from the original nuScenes dataset. We plot the predicted 3D boxes and confidences. Due to the inherent domain gap of BEVDet, the pose estimation of vehicles is not satisfactory. Nevertheless, we can observe a drop in confidence of the non-contact object ($0.672 \rightarrow 0.625$) caused by the adversarial texture, proving the practicality of our method. The result can be further improved by fine-tuning a certain adversarial texture in the current scene.

Furthermore, we compare the effect of our method to strong noise. In Tab.~\ref{tab:comp_strong_noise}, we show the experimental results comparing adversarial NeRF with strong noise in real-world settings. In these experiments, we replace the adversarial texture area with various types of noise, including pure black, the mean color of the background image, and random noise. We observe that adversarial NeRF achieves the lowest predicted confidence and outperforms the other three types of texture in terms of attack performance.

\begin{table*}[h]
    \centering
    % \vspace{-1.0mm}
        \resizebox{0.9\textwidth}{!}{
        \begin{tabular}[width=\linewidth]{lc|cccc}
        \toprule
        \textbf{Texture} & \textbf{Clean} & \textbf{Pure Black} & \textbf{Mean Color} & \textbf{Random Noise} & \textbf{Adversarial NeRF}  \\
        \midrule
        % \midrule
        Confidence	& 0.672 &	0.632 &	0.634 &	0.644	& \textbf{0.625} \\
        \bottomrule
        \end{tabular}
        % \vspace{-.7em}
        }
    \caption{Comparison of strong noise to our attack. }
    % \vspace{-.1em}
    \label{tab:comp_strong_noise}
\end{table*}

% \begin{table*}[t]
% \begin{floatrow}
% \capbtabbox{
%     \begin{tabular}{lcc}
%     \toprule
%     \textbf{Experiments} & \textbf{NDS} & \textbf{mAP} \\
%     \midrule
%      Clean   &   0.3822  &   0.3076  \\ 
%      \midrule
%      Trial 1  &   0.2261   &   0.1322  \\
%      Trial 2   &     0.2263  &   0.1326   \\
%      Trial 3   &     0.2209  &   0.1310 \\
%      Trial 4   &     0.2237  &   0.1302 \\
%      Trial 5   &     0.2228   &  0.1304  \\
%     % \midrule
%      Mean   &     0.2239   &  0.1313  \\
%      Std   &     0.0023   &  0.0011  \\
%     \bottomrule
%     \end{tabular}
% }{
%  \caption{Results of repeatability test.}
%  \label{tab:trial}
% }
% \capbtabbox{
%     \begin{tabular}{lcccccc}
%     \toprule
%     \textbf{Pose} & \textbf{Distribution} &  \textbf{Parameters}   \\
%     \midrule
%     $x$ & Uniform  & $[-5m, 5m]$  \\
%     $y$ & Gaussian  & $\mu = height, \sigma = 0.2$  \\
%     $z$ & Uniform  & $[10m, 15m]$  \\
%     $l$ & Gaussian  & $\mu = l_{mean}, \sigma = 0.5$  \\
%     $w$ & Gaussian  & $\mu = w_{mean}, \sigma = 0.5$  \\
%     $h$ & Gaussian  & $\mu = h_{mean}, \sigma = 0.5$  \\
%     $\theta$ & Gaussian  & $\mu = \pm \pi / 2, \sigma = \pi / 2$  \\
%     \bottomrule
%     \end{tabular}
% }{
%  \caption{Detailed distribution of pose $\mathbf{b}$ in pose sampling.}
%  \label{tab:sam_param}
%  \small
% }
% \end{floatrow}
% \end{table*}

\begin{table}[h]
    \centering
    % \vspace{-1.0mm}
        % \resizebox{\textwidth}{!}{
\begin{tabular}{lcc}
\toprule
\textbf{Number} & \textbf{NDS} & \textbf{mAP} \\
\midrule
 0 (clean)   &   0.3822  &   0.3076  \\ 
 1  &   0.2648   &   0.1895  \\
 2   &     0.2247  &   0.1325   \\
 3   &     0.1749  &   0.0698 \\
\bottomrule
\end{tabular}
        % }
\caption{Ablation of the number of adversarial examples.}
\label{tab:supp_num}
\end{table}

% \begin{table*}[b]
% \begin{floatrow}
% \capbtabbox{
% \begin{tabular}{lcc}
% \toprule
% \textbf{Experiments} & \textbf{NDS} & \textbf{mAP} \\
% \midrule
%  Clean   &   0.3822  &   0.3076  \\ 
%  SUV   &     0.2209  &   0.1310   \\
%  SUV to Sedan  &   0.2344   &   0.1449  \\
%  SUV to Hatchback  &  0.2319  &   0.1413   \\
%  SUV to Jeep   &     0.2348  &   0.1452 \\
% \bottomrule
% \caption{Transfer to unseen instance}
% \end{tabular}
% }{
%  \caption{Results of our adversarial texture transfer to unseen shape.}
%  \label{tab:transfer_instance}
% }
% \capbtabbox{
% \begin{tabular}{lcc}
% \toprule
% \textbf{Number} & \textbf{NDS} & \textbf{mAP} \\
% \midrule
%  0 (clean)   &   0.3822  &   0.3076  \\ 
%  1  &   0.2648   &   0.1895  \\
%  2   &     0.2247  &   0.1325   \\
%  3   &     0.1749  &   0.0698 \\
% \bottomrule
% \end{tabular}
% }{
%  \caption{Ablation of the number of adversarial examples.}
%  \label{tab:supp_num}
%  \small
% }
% \end{floatrow}
% \end{table*}

\section{Ablation of The Number of Adversarial Examples}\label{num_adv}

% \begin{wraptable}[11]{r}{0.3\textwidth}
% \vspace{-5mm}
% \resizebox{0.9\linewidth}{!}{
% \begin{tabular}{lcc}
% \toprule
% \textbf{Number} & \textbf{NDS} & \textbf{mAP} \\
% \midrule
%  0   &   0.3822  &   0.3076  \\ 
%  1  &   0.2648   &   0.1895  \\
%  2   &     0.2247  &   0.1325   \\
%  3   &     0.1749  &   0.0698 \\
% \bottomrule
% \end{tabular}
% \vspace{-5mm}
% \caption{
% }
% \label{ablation_volsub_imgres}
% }
% \end{wraptable}

% % \begin{table}[h!]
%     \centering
%     \resizebox{1\textwidth}{!}{
%     \begin{tabular}{lcc}
    % \toprule
    % \textbf{Number} & \textbf{NDS} & \textbf{mAP} \\
    % \midrule
    %  0   &   0.3822  &   0.3076  \\ 
    %  1  &   0.2648   &   0.1895  \\
    %  2   &     0.2247  &   0.1325   \\
    %  3   &     0.1749  &   0.0698 \\
    % \bottomrule
    % \end{tabular}
%     }
%     \label{tab:1}
%     \caption{.}
% % \vspace{-4.0mm}
% % \end{table}

Since the number of populated adversarial examples is related to the area of adversarial texture, we ablate the number of rendered adversarial examples per image in Tab.~\ref{tab:supp_num}. We observe that the more adversarial objects, the better the attack performance. The number 0 denotes a clean evaluation without attacks. In all experiments in our main paper except Sec. 5.2, we render two adversarial examples for evaluation to avoid overcrowded scenes. We note that for number $>1$, the rendered adversarial patches are from the same adversarial example, since we only maintain a single adversarial object during training.

\section{Adversarial Texture Transfer to Unseen Vehicle}\label{trans_unseen}
To further validate the transferability of our method, we analyze the attack performance of a trained adversarial texture transfer to an unseen shape. As shown in Tab.~\ref{tab:transfer_instance}, we train our adversarial examples using only an SUV-type vehicle and then transfer the adversarial texture to other unseen vehicles by our proposed disentangled texture and shape generation. The target types of vehicles include Sedan, Hatchback, and Jeep. The transfer results of the unseen types of vehicles show comparable attack performance compared with the seen one, which demonstrates the transferability of our adversarial texture to unseen shapes. The rendered images of adversarial examples can be found in Fig.~\ref{fig:sedan}-\ref{fig:jeep}.

\begin{table}[h]
    \centering
    % \vspace{-1.0mm}
        % \resizebox{\textwidth}{!}{
\begin{tabular}{lcc}
\toprule
\textbf{Experiments} & \textbf{NDS} & \textbf{mAP} \\
\midrule
 Clean   &   0.3822  &   0.3076  \\ 
 SUV   &     0.2209  &   0.1310   \\
 SUV to Sedan  &   0.2344   &   0.1449  \\
 SUV to Hatchback  &  0.2319  &   0.1413   \\
 SUV to Jeep   &     0.2348  &   0.1452 \\
\bottomrule
\end{tabular}
        % }
\caption{Transfer to unseen instance}
\label{tab:transfer_instance}
\end{table}

\section{Repeatability Tests}\label{repe_test}

In our pose sampling, we randomly and independently sample the parameters of the pose for each frame from pose distribution $\mathcal{B}$. In this section, we investigate the impact of the randomness of pose sampling. We conduct five independent evaluations using the same trained adversarial example and show results in Tab.~\ref{tab:trial}. We found that regardless of the random pose sampling, all the trials display a similar attack performance. The results indicate that our adversarial attack is robust against the randomness of pose sampling.

\begin{table}[h]
    \centering
    % \vspace{-1.0mm}
        % \resizebox{\textwidth}{!}{

    \begin{tabular}{lcc}
    \toprule
    \textbf{Experiments} & \textbf{NDS} & \textbf{mAP} \\
    \midrule
     Clean   &   0.3822  &   0.3076  \\ 
     \midrule
     Trial 1  &   0.2261   &   0.1322  \\
     Trial 2   &     0.2263  &   0.1326   \\
     Trial 3   &     0.2209  &   0.1310 \\
     Trial 4   &     0.2237  &   0.1302 \\
     Trial 5   &     0.2228   &  0.1304  \\
    % \midrule
     Mean   &     0.2239   &  0.1313  \\
     Std   &     0.0023   &  0.0011  \\
    \bottomrule
    \end{tabular}
        % \vspace{-.7em}
        % }
    \caption{Results of repeatability test.}
    % \vspace{-.1em}
    \label{tab:trial}
\end{table}

\section{Impact of the Perceptibility of the Attack}\label{perceptibility}
We conduct experiments investigating the influence of distance and pixel proportion. In the setting of 3D vision, the farther the distance, the smaller the pixel proportion (size of patch / (1600*900)), thus less perceptible. From Tab.~\ref{tab:percept_tab}, we can observe that as the distance increases, the pixel proportion decreases and the attack performance relatively decreases as well. This indicates that the higher the perceptibility (larger pixel proportion), the better the attack performance.

\begin{table*}[h]
    \centering
    \vspace{-1.0mm}
        \resizebox{0.68\textwidth}{!}{
        \begin{tabular}[width=\linewidth]{l|ccccc}
        \toprule
        \textbf{Distance (m)} & \textbf{10} & \textbf{11} & \textbf{12} & \textbf{13} & \textbf{14}  \\
        \midrule
        % \midrule
        Pixel proportion $(\%)$ & 4.67   & 3.67 & 2.96 & 2.42 & 2.04  \\
        Performance drop $(\%)$  & 41.47  & 39.56 & 37.11 & 34.74 & 32.52  \\
        \bottomrule
        \end{tabular}
        % \vspace{-.7em}
        }
    \caption{Influence of perceptibility to our attacks}
    % \vspace{-.1em}
    \label{tab:percept_tab}
\end{table*}

\section{Limitation and Future Work}\label{sec:limit}

\myparagraph{Learning to Sample and Attack} As we do not have access to the dataset annotations, we can not model the explicit relationship between adversarial and normal objects to avoid collision, and the collision itself can cause a performance drop ("No Parts" in Tab.3 of the main paper). Future work can apply geometry-aware composition~\cite{chen2021geosim} to mitigate this problem. Additionally, future research can explore learning to predict optimal poses of adversarial objects to maximize the effectiveness of attacks.

\myparagraph{Broader Impact} The recent development of NeRF has led to remarkable progress in NeRF-based driving scene simulation~\cite{yang2023unisim,lift3D2023CVPR,li2022climatenerf}. Our adversarial framework is general and can be extended to integrate with the advances in NeRF-based simulators to benefit a wide spectrum of practical systems. For instance, our framework can be combined with UniSim~\cite{yang2023unisim} to perform adversarial closed-loop evaluations of self-driving cars in NeRF environments, or with ClimateNeRF~\cite{li2022climatenerf} to identify adverse weather conditions that may corrupt the autonomous driving system. We believe that our work provides valuable insights and opens up new possibilities for creating authentic adversarial evaluations that improve the robustness of self-driving cars.

\myparagraph{Potential Harmful Consequences} The trained adversarial examples have the potential to induce serious traffic accidents in driving scenarios. However, our work is not intended to cause disruptions in autonomous driving systems. Instead, our goal is to use the examples to gain a deeper understanding of the systems and improve their robustness. We hope our work will draw more attention of the community to further verify and enhance the robustness of autonomous driving systems.

\section{Additional Qualitative Results}\label{qua_result}

In this section, we present additional qualitative results of our trained adversarial example. In Fig.~\ref{fig:suv_part}, we show rendered images of an SUV-type adversarial example, and different parts of semantic-guided regularization. Then we display rendered images of adversarial texture transfer to the unseen vehicles in Fig.~\ref{fig:sedan}-\ref{fig:jeep}.

\begin{figure*}[h!]
    \centering
    \includegraphics[width = 1\textwidth, trim = 0 0 0 0, clip]{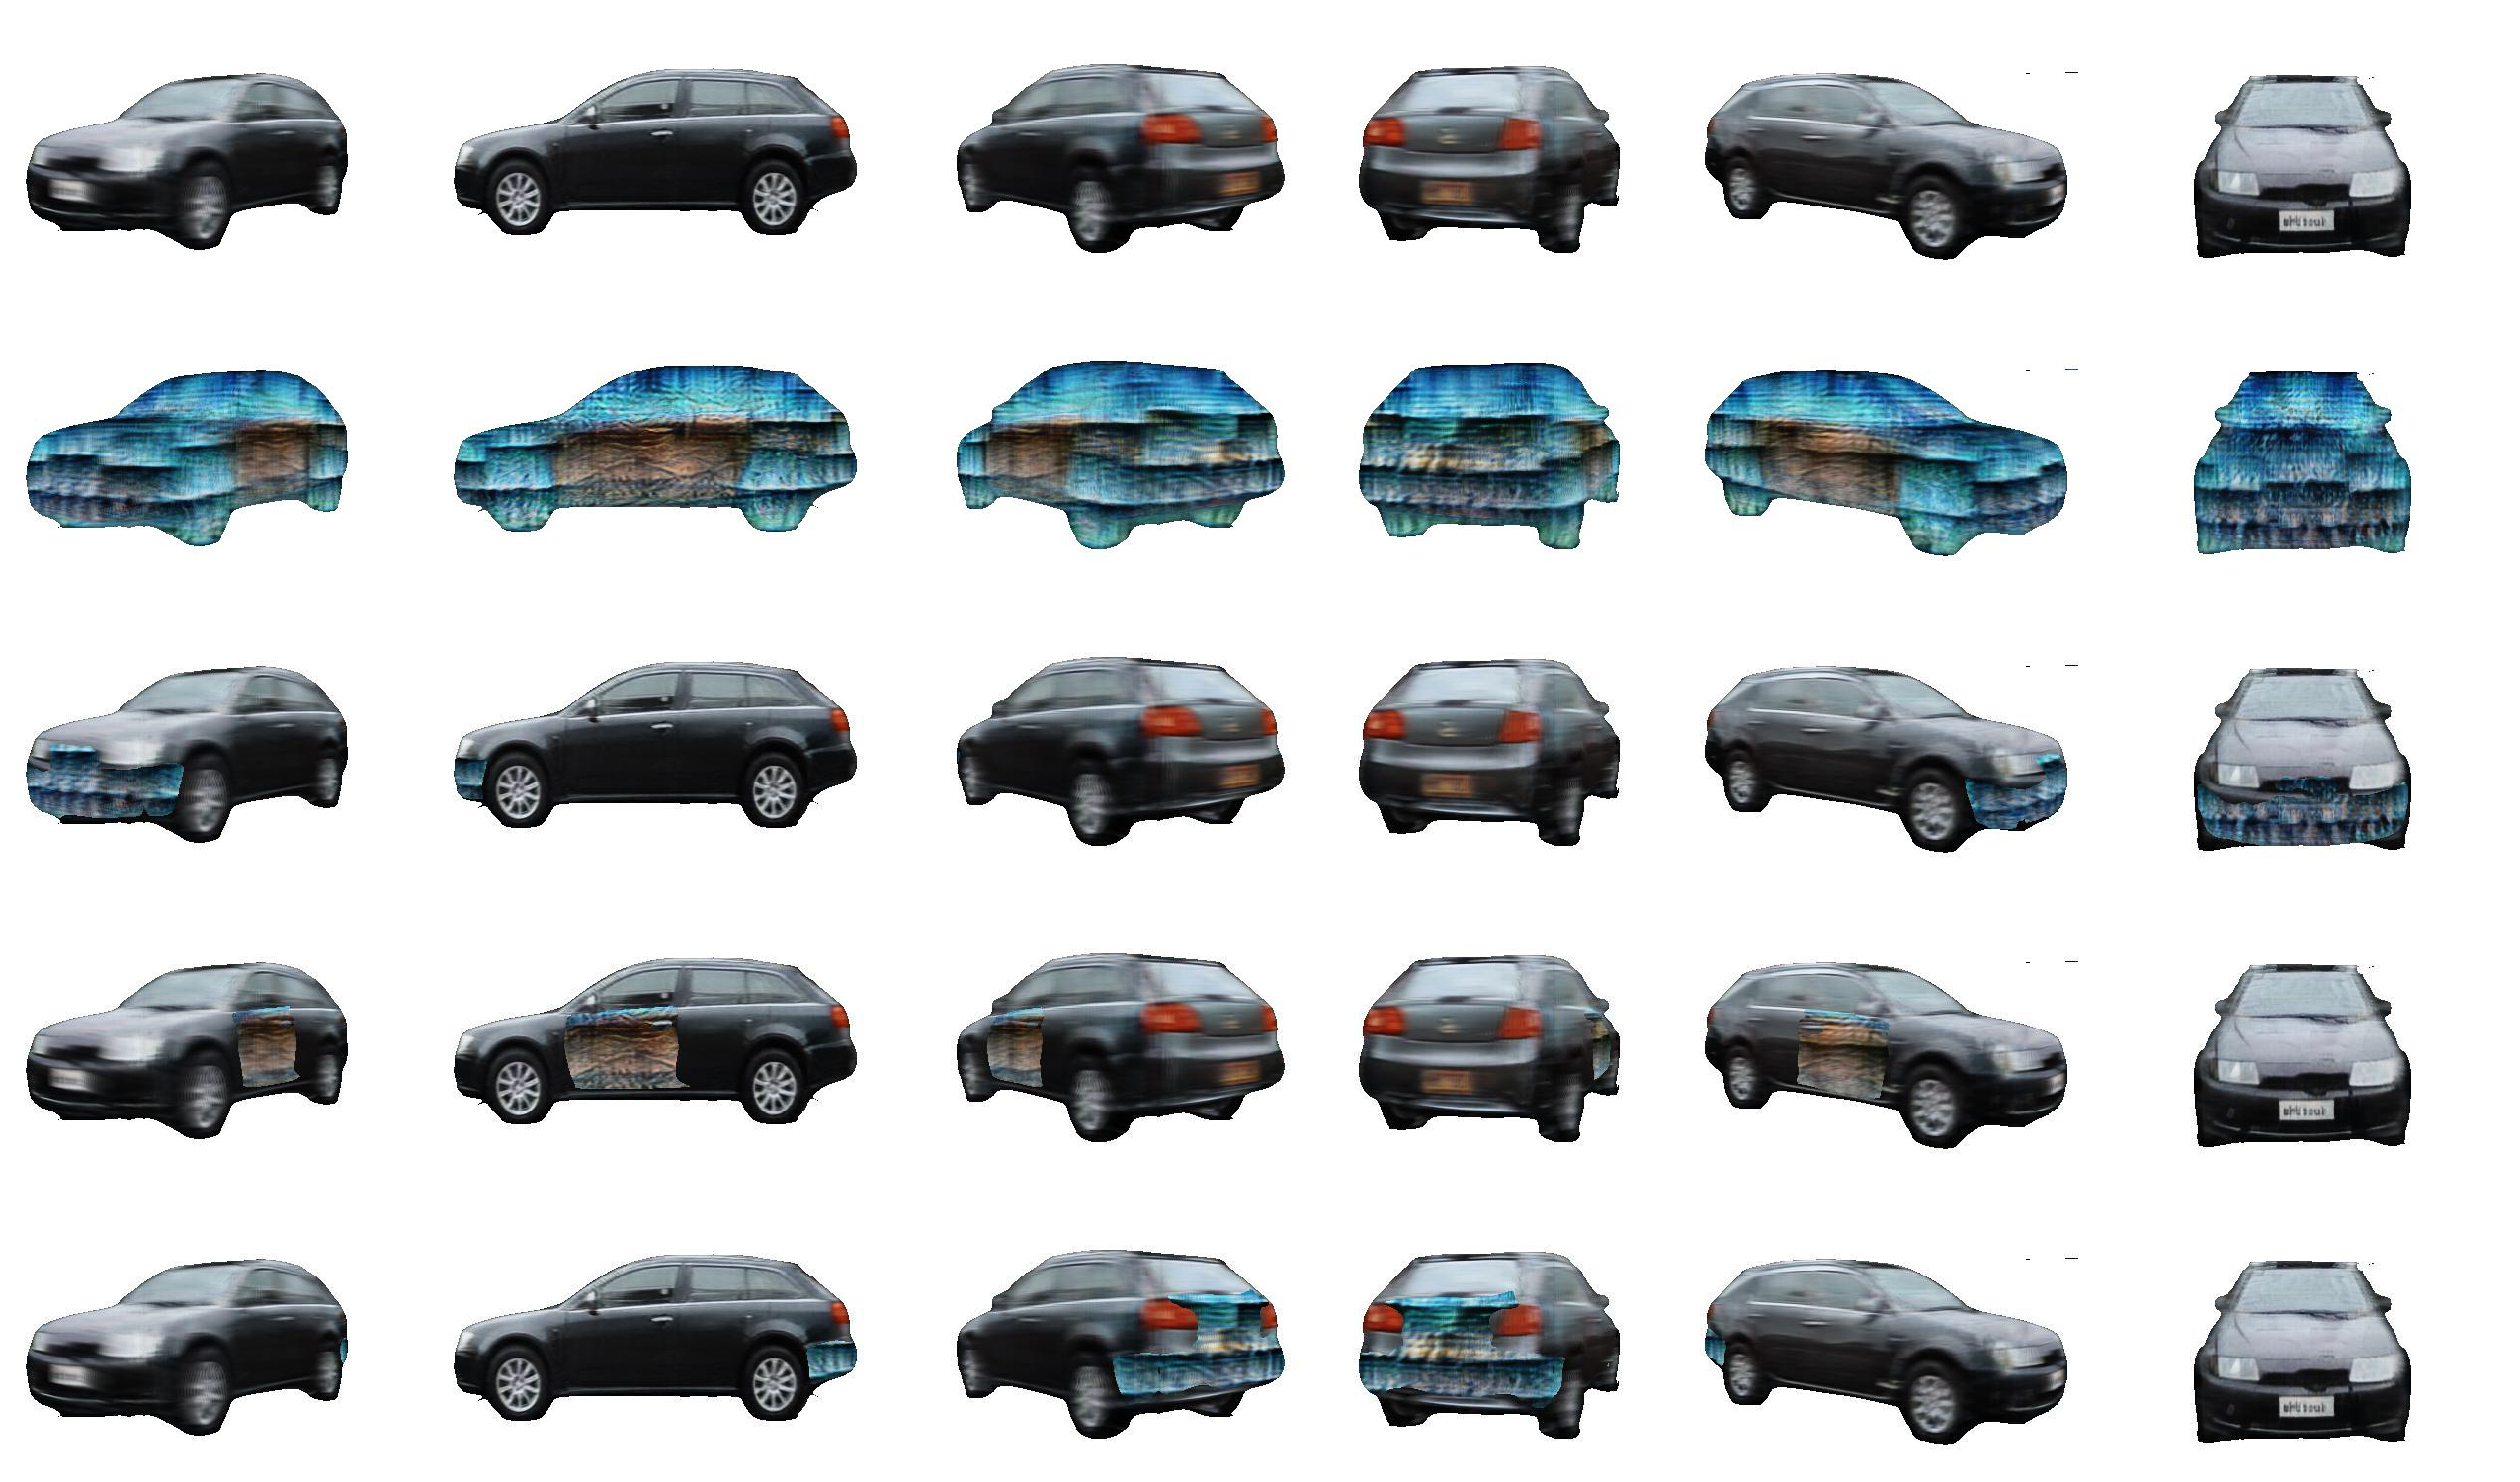}
    \caption{
    \textbf{First row:} the initial SUV-type vehicle. \textbf{Second row:} the trained full-part adversarial example using the SUV-type vehicle. \textbf{Third row to the fifth row:} The results of full part adversarial texture transfer to the front part, side part, and rear part.
    }
    \label{fig:suv_part}
\end{figure*}

\begin{figure*}[h!]
    \centering
    \includegraphics[width = 1\textwidth, trim = 0 0 0 0, clip]{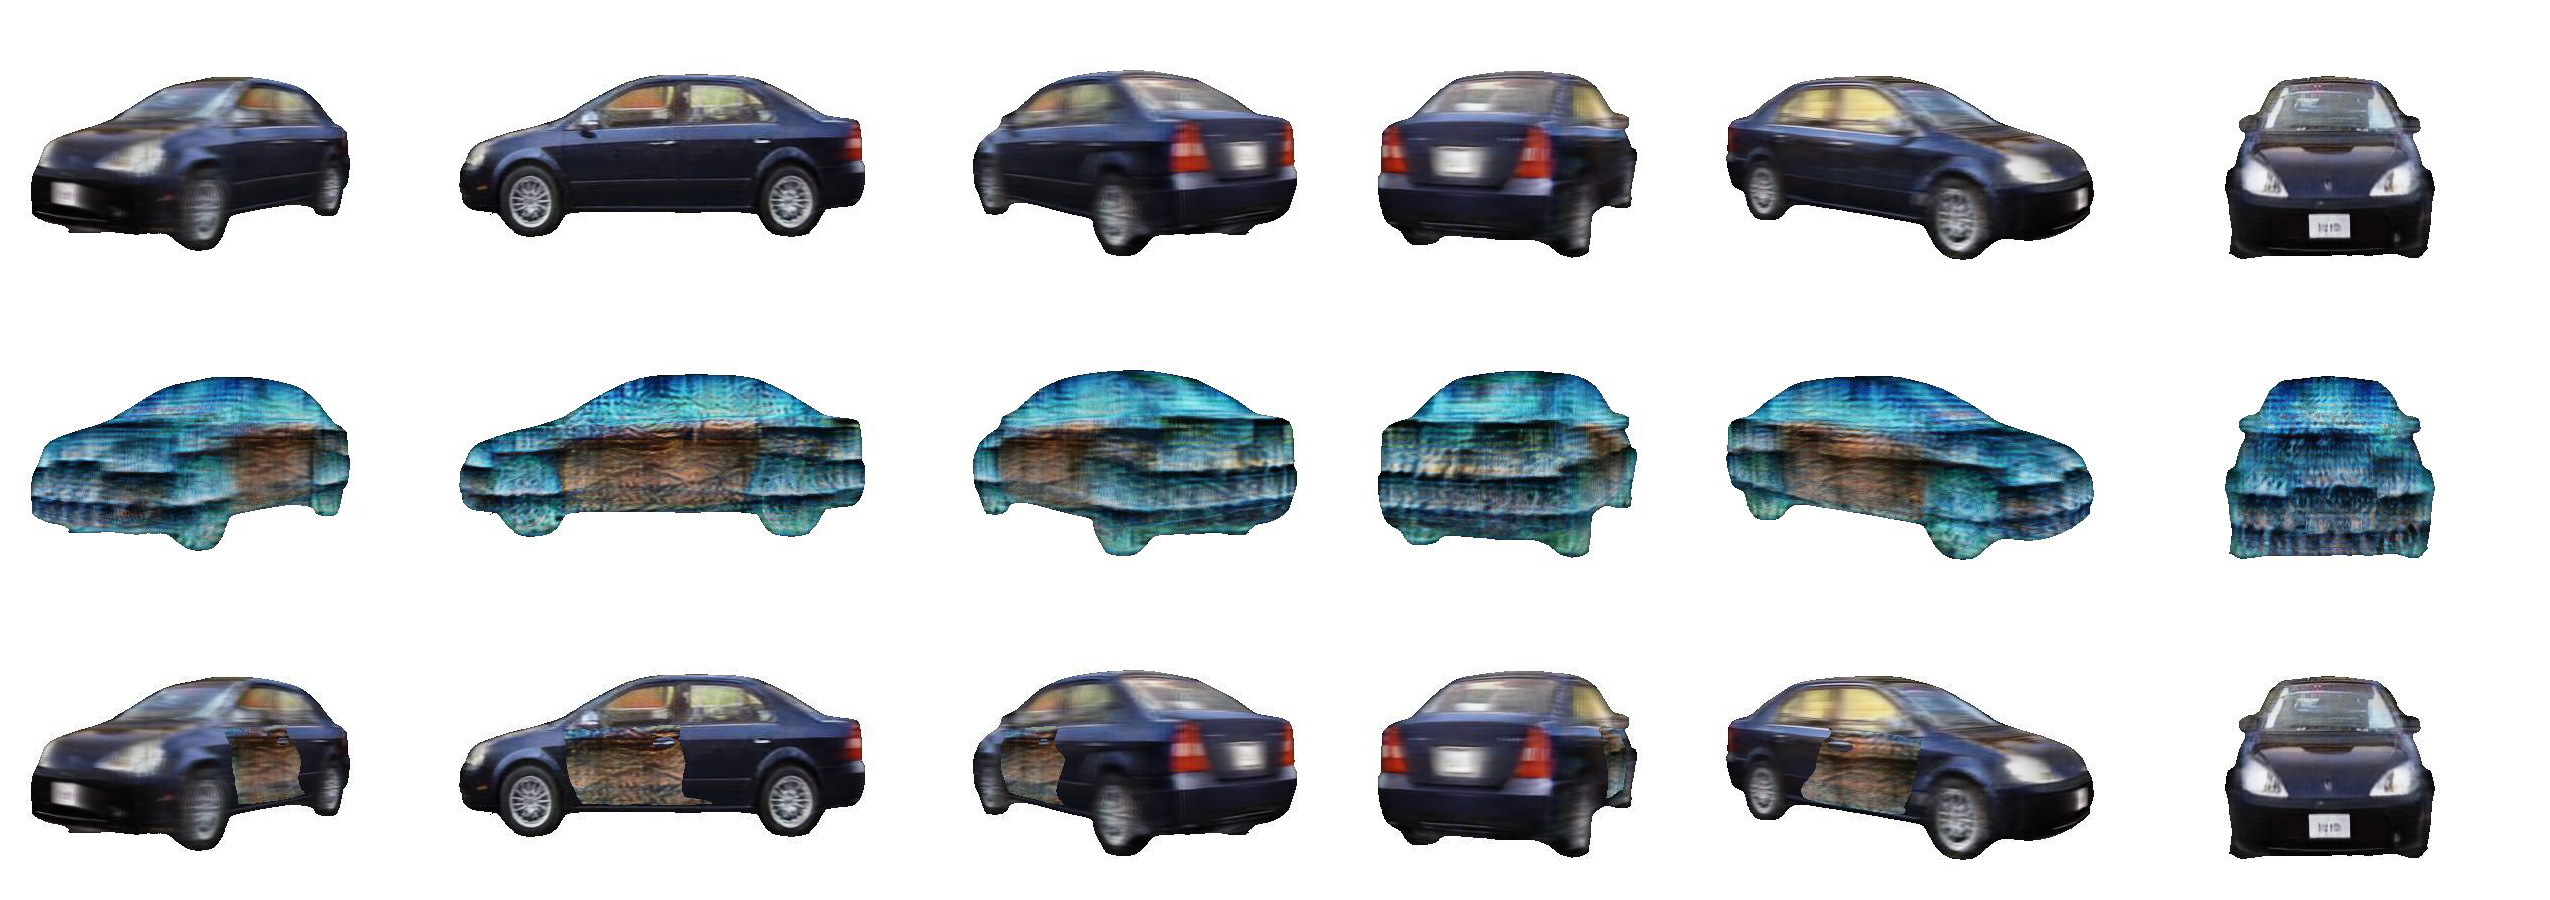}
    \caption{
    \textbf{First row:} Rendered images of a Sedan-type vehicle. \textbf{Second and third rows:} We transfer the trained adversarial texture of an SUV-type vehicle (Fig.~\ref{fig:suv_part}) to the Sedan-type vehicle.
    }
    \label{fig:sedan}
\end{figure*}

% \newpage
% \clearpage

\begin{figure*}[h!]
    \centering
    \includegraphics[width = 1\textwidth, trim = 0 0 0 0, clip]{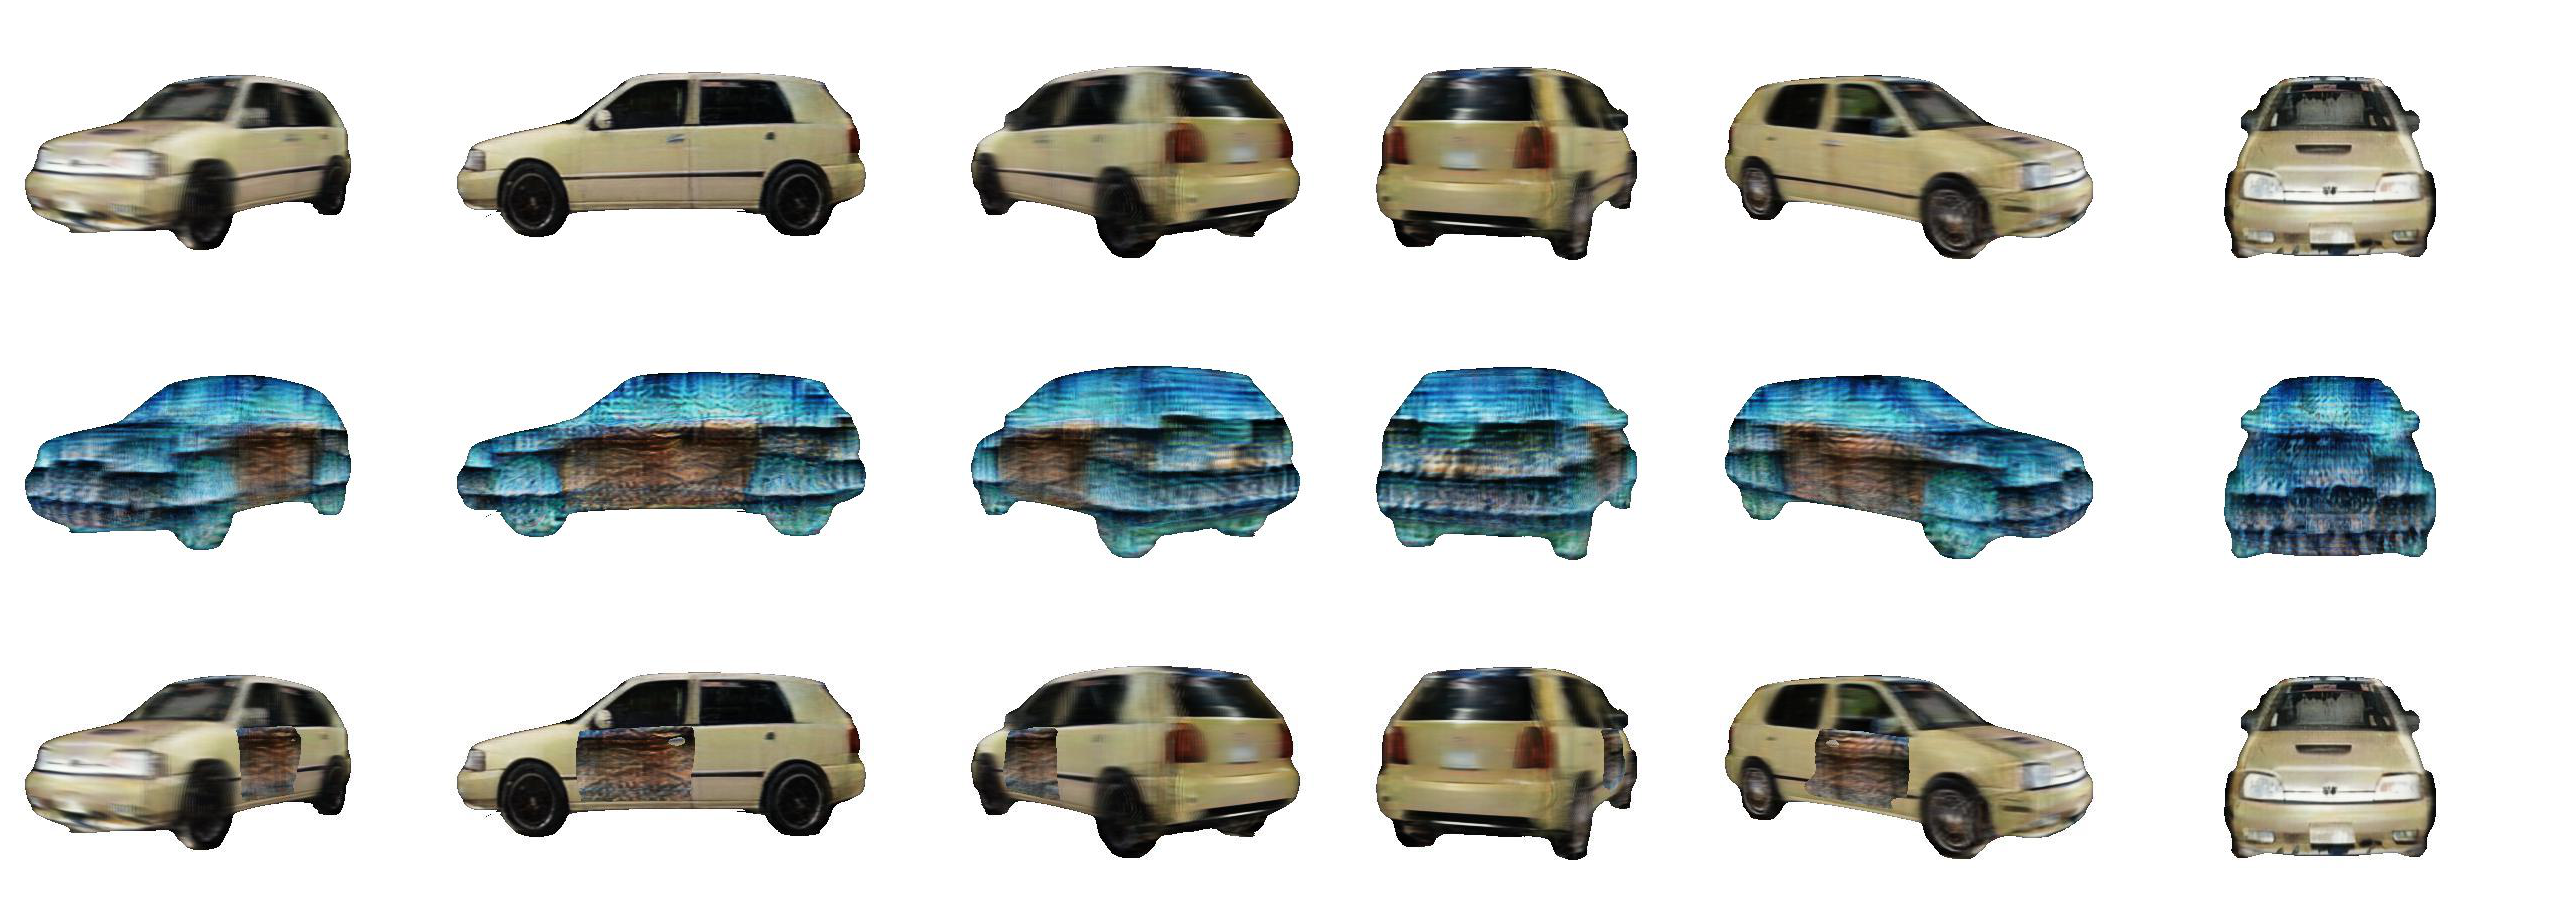}
    \caption{
    \textbf{First row:} Rendered images of a Hatchback-type vehicle. \textbf{Second and third rows:} We transfer the trained adversarial texture of an SUV-type vehicle (Fig.~\ref{fig:suv_part}) to the Hatchback-type vehicle.
    }
    \label{fig:hatch}
\end{figure*}

\begin{figure*}[h!]
    \centering
    \includegraphics[width = 1\textwidth, trim = 0 0 0 0, clip]{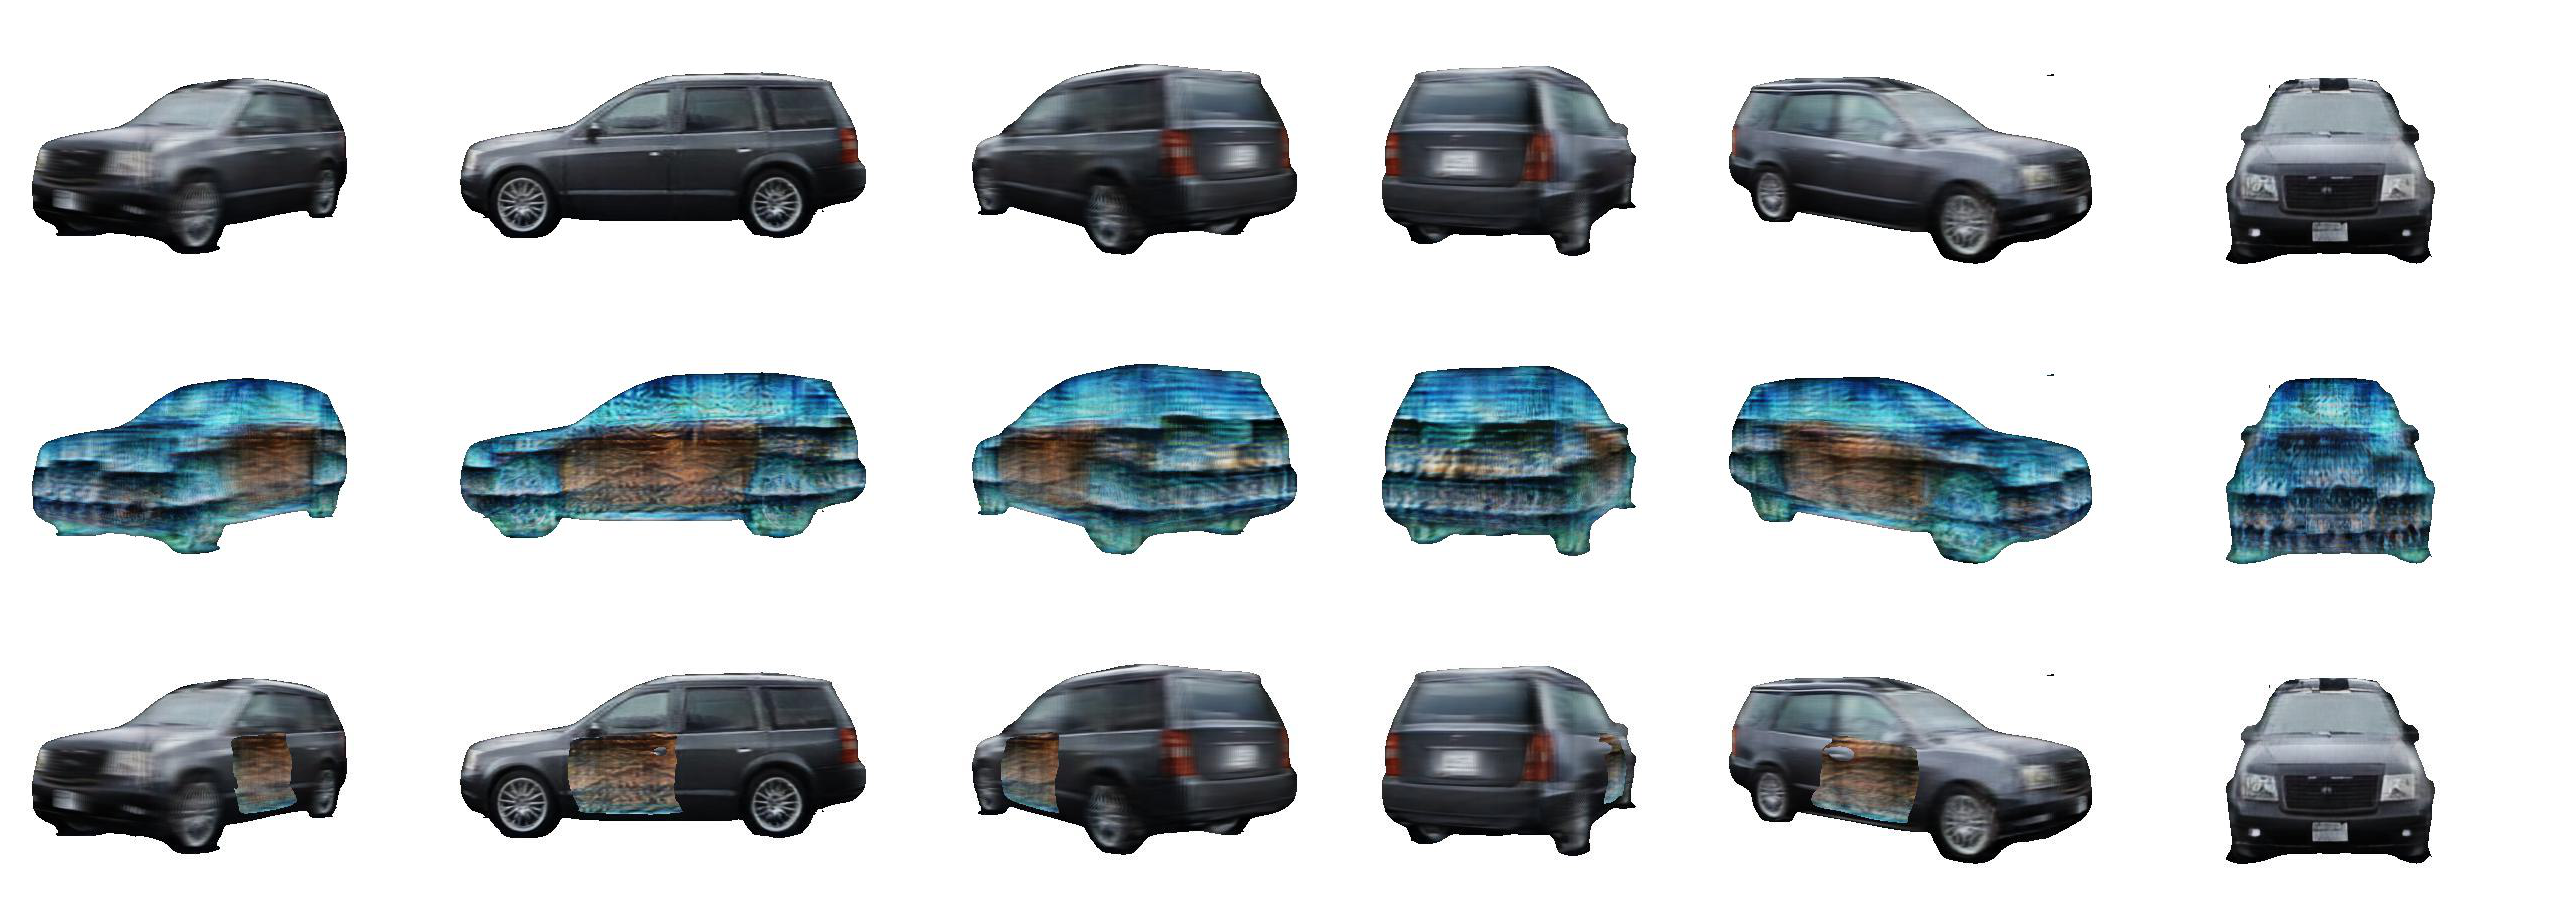}
    \caption{
    \textbf{First row:} Rendered images of a Jeep-type vehicle. \textbf{Second and third rows:} We transfer the trained adversarial texture of an SUV-type vehicle (Fig.~\ref{fig:suv_part}) to the Jeep-type vehicle.
    }
    \label{fig:jeep}
\end{figure*}
